# Supplementary material for: Linear Query Approximation Algorithms for Non-monotone Submodular Maximization under Knapsack Constraint
Source: arXiv:2305.10292 source file (2026-11-26)
Supplement: Supplementary file 1 [file SMK-IJCAI23-Camera_Ready_NoAppendix.pdf]

# Linear Query Approximation Algorithms for Non-monotone Submodular Maximization under Knapsack Constraint

Canh V. Pham<sup>1\*</sup>, Tan D. Tran<sup>2</sup>, Dung T. K. Ha<sup>2</sup> and My T. Thai<sup>3</sup>

<sup>1</sup>ORLab, Faculty of Computer Science, Phenikaa University, Hanoi, Vietnam

<sup>2</sup> Faculty of Information Technology, VNU University of Engineering and Technology, Hanoi, Vietnam

<sup>3</sup>Department of Computer and Information Science and Engineering  
University of Florida, Gainesville, Florida 32611

canh.phamvan@phenikaa-uni.edu.vn, {22027005, 20028008}@vnu.edu.vn, mythai@cise.ufl.edu

## Abstract

This work, for the first time, introduces two constant factor approximation algorithms with linear query complexity for non-monotone submodular maximization over a ground set of size  $n$  subject to a knapsack constraint, DLA and RLA. DLA is a deterministic algorithm that provides an approximation factor of  $6+\epsilon$  while RLA is a randomized algorithm with an approximation factor of  $4+\epsilon$ . Both run in  $O(n \log(1/\epsilon)/\epsilon)$  query complexity. The key idea to obtain a constant approximation ratio with linear query lies in: (1) dividing the ground set into two appropriate subsets to find the near-optimal solution over these subsets with linear queries, and (2) combining a threshold greedy with properties of two disjoint sets or a random selection process to improve solution quality. In addition to the theoretical analysis, we have evaluated our proposed solutions with three applications: Revenue Maximization, Image Summarization, and Maximum Weighted Cut, showing that our algorithms not only return comparative results to state-of-the-art algorithms but also require significantly fewer queries.

## 1 Introduction

In the variety of submodular optimization, Submodular Maximization under a Knapsack (SMK) constraint is one of the most fundamental problems. In this problem, given a ground set  $V$  of size  $n$  and a non-negative submodular set function  $f : 2^V \mapsto \mathbb{R}_+$ . Assume that each element  $e \in V$  has a positive cost  $c(e)$  and there is a budget  $B$ , SMK asks for finding  $S \subseteq V$  subject to  $c(S) = \sum_{e \in S} c(e) \leq B$  that maximizes  $f(S)$ . SMK captures important constraints in practical applications, such as bounds on costs, time, or size, thereby attracting a lot of attention recently [Mirzasoleiman *et al.*, 2016; Amanatidis *et al.*, 2021; Han *et al.*, 2021; Sviridenko, 2004; Li *et al.*, 2022; Ene and Nguyen, 2019; Lee *et al.*, 2010a; Amanatidis *et al.*, 2020; Gupta *et al.*, 2010].

In addition to obtaining a near-optimal solution to SMK, designing such a solution also focuses on reducing query

complexity, especially in an era of big data. With an explosion of input data, the search space for a solution has increased exponentially. Unfortunately, submodularity requires an algorithm to evaluate the objective function whenever observing an incoming element. Therefore, it is necessary to design efficient algorithms that reduce the number of queries to linear or nearly linear.

Furthermore, to model SMK for real-world applications, the objective functions may be non-monotone, since the marginal contribution of an element to a set may not always increase. Notable examples with non-monotone objective functions can be found in revenue maximization on social network [Mirzasoleiman *et al.*, 2016; Kuhnle, 2019], image summarization with a representative [Mirzasoleiman *et al.*, 2016] or maximum weight cut [Amanatidis *et al.*, 2020].

Unfortunately, no constant approximation algorithm with linear query complexity exists for non-monotone SMK compared to its counterpart. For the monotone SMK, the best approximation factor of  $e/(e-1)$  is achieved within  $O(n^5)$  number of queries [Sviridenko, 2004]; and the fastest algorithm has a factor of  $2+\epsilon$  needs a linear number of queries [Li *et al.*, 2022]. But for non-monotone, the best approximation algorithm needs polynomial queries and has a factor of  $1/0.385$  [Buchbinder and Feldman, 2019] and the fastest algorithm with constant factor requires near-linear query complexity of  $O(n \log k)$ , where  $k$  is the maximum cardinality of any feasible solution to SMK [Han *et al.*, 2021]. Thus this work aims to close this gap by addressing the following open question: *Is there a constant factor approximation algorithm for non-monotone SMK in linear query complexity?*

Solving non-monotone SMK with linear query complexity is more challenging than that of the monotone case due to the following reasons. First, the property of the monotone submodular function plays an important role in analyzing the theoretical bound of an obtained solution. Second, algorithms for the non-monotone case need more queries to obtain information from all elements in the condition that the marginal contribution of an element may be negative.

**Our Contributions.** To tackle the above challenges, we propose two approximation algorithms, DLA and RLA, that achieve a constant factor approximation, yet both require linear query complexity. Our DLA is a deterministic algorithm with an approximation factor of  $6+\epsilon$  within  $O(n \log(1/\epsilon)/\epsilon)$

---

\*Corresponding author

| Reference                                         | Approximation factor | Query Complexity                 | Deterministic/Randomized |
|---------------------------------------------------|----------------------|----------------------------------|--------------------------|
| [Mirzasoleiman <i>et al.</i> , 2016] (FANTOM)     | $10 + \epsilon$      | $O(n^2 \log(n)/\epsilon)$        | Randomized               |
| [Amanatidis <i>et al.</i> , 2020] (SAMPLE GREEDY) | $5.83 + \epsilon$    | $O(n \log(n/\epsilon)/\epsilon)$ | Randomized               |
| [Han <i>et al.</i> , 2021] (SMKDETACC)            | $6 + \epsilon$       | $O(n \log(k/\epsilon)/\epsilon)$ | Deterministic            |
| [Han <i>et al.</i> , 2021] (SMKSTREAM)            | $6 + \epsilon$       | $O(n \log(B)/\epsilon)$          | Deterministic            |
| [Han <i>et al.</i> , 2021] (SMKRANACC)            | $4 + \epsilon$       | $O(n \log(k/\epsilon)/\epsilon)$ | Randomized               |
| DLA (Algorithm 3, this paper)                     | $6 + \epsilon$       | $O(n \log(1/\epsilon)/\epsilon)$ | Deterministic            |
| RLA (Algorithm 4, this paper)                     | $4 + \epsilon$       | $O(n \log(1/\epsilon)/\epsilon)$ | Randomized               |

Table 1: Fastest algorithms for non-monotone SMK problem, where  $k$  is the maximum cardinality of any feasible solution to SMK.

queries. Therefore, DLA is significantly faster than the deterministic algorithm of [Han *et al.*, 2021], which achieved the best-known approximation factor for  $6 + \epsilon$  with nearly-linear query complexity of  $O(n \log(k/\epsilon)/\epsilon)$ . RLA is a randomized algorithm that achieves a factor of  $4 + \epsilon$  in  $O(n \log(1/\epsilon)/\epsilon)$  queries. Therefore, RLA achieves the same factor of the randomized algorithm as in [Han *et al.*, 2021], which currently provides the best approximation factor in near-linear query complexity of  $O(n \log(k/\epsilon)/\epsilon)$ . Note that  $k$  may be as large as  $n$ , so the query complexity of the algorithms in [Han *et al.*, 2021] can be  $O(n \log(n/\epsilon)/\epsilon)$ . Table 1 compares the performance of our algorithms with that of existing fast algorithms.

Both our algorithms focus on a novel algorithmic approach that consists of two components: (1) dividing the ground set into two appropriate subsets and finding the approximation solution over these subsets with linear queries, and (2) combining the threshold greedy procedure developed by [Badanidiyuru and Vondrák, 2014] with two disjoint candidate solutions (for DLA) or a random process (for RLA) to construct serial candidate solutions to give better theoretical bounds. At the heart of the first component, we adapt the method of simultaneously constructing two disjoint sets, which is first introduced by [Han *et al.*, 2020; Amanatidis *et al.*, 2022] and later used by [Sun *et al.*, 2022; Han *et al.*, 2021] to bound the utility of candidate solutions. By incorporating a method of dividing the ground set into two reasonable subsets, we can bound the cost of feasible solutions, thereby obtaining a constant approximation factor within only a one-time scan over these subsets. In the second component, we adapt the threshold greedy, where thresholds are adjusted accordingly to provide a constant number of candidate solutions. Finally, we boost the solution quality of our algorithm by re-scanning the best elements for selecting candidate solutions without increasing query complexity.

Extensive experiments show that our algorithms outperform several state-of-the-art algorithms [Mirzasoleiman *et al.*, 2016; Amanatidis *et al.*, 2021; Han *et al.*, 2021] regarding solution quality and the number of queries. In particular, DLA provides the best solution quality and needs fewer queries than the faster approximation deterministic algorithm in [Han *et al.*, 2021], while RLA returns competitive solutions but needs the fewest queries.

**Paper Organization.** The rest of the paper is structured as follows. Section 2 provides the literature review on non-monotone SMK problem. Notations are presented in Section 3. Section 4 introduces our proposed algorithms and theoretical analysis. Experimental computation is provided in Section 5. Finally, we conclude this work in Section 6.

## 2 Related Works

In this section, we review the related work for the non-monotone SMK problem only. A brief review of monotone SMK and submodular maximization subject to cardinality, a special cases of SMK, can be found in the Appendix.

Randomization is one of the effective methods for designing approximation algorithms for submodular non-monotone SMK. The first randomized algorithm was proposed by [Lee *et al.*, 2010b] with a factor of  $5 + \epsilon$ ; the factor was later improved to  $4 + \epsilon$  by [Kulik *et al.*, 2013]. Several researchers tried to enhance the approximation factor to  $e/(e - 1) + \epsilon$  or  $e + \epsilon$  [Chekuri *et al.*, 2014; Feldman *et al.*, 2011; Ene and Nguyen, 2019; Buchbinder and Feldman, 2019]. The best factor in this line of randomized algorithms was  $1/0.385 \approx 2.6$  due to [Buchbinder and Feldman, 2019], using the multi-linear extension method with the rounding scheme technique in [Kulik *et al.*, 2013]. However, this work has to handle complicated multi-linear extensions and uses a large number of queries. In contrast, [Amanatidis *et al.*, 2020] proposed a sample greedy, a fast algorithm with a factor of  $5.83 + \epsilon$  requiring  $O(n \log(n/\epsilon)/\epsilon)$  queries. An efficient parallel algorithm with a factor of  $9.465 + \epsilon$  was introduced by [Amanatidis *et al.*, 2021], but it needed a high query complexity of  $O(n^2 \log^2(n) \log(1/\epsilon)/\epsilon^3)$ . Significantly, [Han *et al.*, 2021] introduced the current fastest randomized algorithm with the factor of  $4 + \epsilon$  in  $O(n \log(k/\epsilon)/\epsilon)$  queries.

For the deterministic algorithm approach, [Gupta *et al.*, 2010] first presented a deterministic algorithm with a factor of 6. Their algorithm modified Sviridenko’s algorithm [Sviridenko, 2004] and combined with an algorithm for unconstrained non-monotone submodular maximization [Buchbinder *et al.*, 2015]; however, it took  $O(n^5)$  query complexity. Since then, there are several algorithms have been proposed to reduce the number of queries. The FANTOM algorithm [Mirzasoleiman *et al.*, 2016] improved the query complexity to  $O(n^2 \log(n)/\epsilon)$  but returned a larger factor of 10. Algorithm of [Li, 2018] achieved a factor of  $9.5 + \epsilon$  in  $O(nk) \max\{\epsilon^{-1}, \log \log n\}$  and it can be used for  $p$ -system and  $d$ -knapsack constraints. [Cui *et al.*, 2021] introduced a streaming algorithm with a factor of  $2.05 + \rho_{\text{Alg}}$  in  $O((n + T_{\text{Alg}(k)}) \log B)$  queries, where  $\rho_{\text{Alg}}$  was the approximation factor any offline algorithm Alg for SMK and  $T_{\text{Alg}(k)}$  was the query complexity of Alg with  $k$  input elements. The factor and query complexity of the algorithm are quite large because they depend on  $\rho_{\text{Alg}}$  and  $k$  can be as large as  $n$ . Recently, [Han *et al.*, 2021] also presented another one that was deterministic

the factor of  $6 + \epsilon$  in nearly-linear queries  $O(n \log(k/\epsilon)/\epsilon)$ . Currently, the best approximation factor of a deterministic algorithm for non-monotone SMK is due to [Sun *et al.*, 2022] achieving an approximation factor of  $4 + \epsilon$  but requiring an impractical query complexity of  $O(n^3 \log(n/\epsilon)/\epsilon)$ .

### 3 Preliminaries

We use the definition of submodularity based on *the diminishing return property*: A set function  $f : 2^V \mapsto \mathbb{R}_+$ , defined on all subsets of a ground set  $V$  of size  $n$  is submodular iff for any  $A \subseteq B \subseteq V$  and  $e \in V \setminus B$ , we have:

$$f(A \cup \{e\}) - f(A) \geq f(B \cup \{e\}) - f(B).$$

Each element  $e \in V$  is assigned a positive cost  $c(e) > 0$ , and the total cost of a set  $S \subseteq V$  is a modular function, i.e.,  $c(S) = \sum_{e \in S} c(e)$ . Given a budget  $B$ , we assume that every item  $e \in V$  satisfies  $c(e) \leq B$ ; otherwise, we can simply discard it. The SMK problem is to determine:

$$\arg \max_{S \subseteq V: c(S) \leq B} f(S). \quad (1)$$

We denote an instance of SMK by a tuple  $(f, V, B)$ . For simplicity, we assume that  $f$  is non-negative, i.e.,  $f(X) \geq 0$  for all  $X \subseteq V$  and normalized, i.e.,  $f(\emptyset) = 0$ . We define the contribution gain of an element  $e$  to a set  $S \subseteq V$  as  $f(e|S) = f(S \cup \{e\}) - f(S)$  and we write  $f(\{e\})$  as  $f(e)$  for any  $e \in V$ . We assume that there exists an oracle query, which when queried with the set  $S$  returns the value  $f(S)$ .

We denote  $O$  as an optimal solution with the optimal value  $\text{opt} = f(O)$  and  $r = \arg \max_{o \in O} c(o)$ . Another frequently used property of a non-negative submodular function is: For any  $T \subseteq V$  and two disjoint subsets  $X, Y$  of  $V$  we have:

$$f(T) \leq f(T \cup X) + f(T \cup Y). \quad (2)$$

We use this Lemma to analyze our algorithms' performance.

**Lemma 1.** (Lemma 2.2. in [Buchbinder *et al.*, 2014]) Let  $f : 2^V \mapsto \mathbb{R}_+$  be submodular. Denote by  $A(p)$  a random subset of  $A$  where each element appears with probability at most  $p$  (not necessary independently). Then  $\mathbb{E}[f(A(p))] \geq (1 - p)f(\emptyset)$ .

## 4 Proposed Algorithms

In this section, we introduce two main algorithms, DLA and RLA. The core of these two algorithms lies in our novel design of LA (Linear Approximation), a 19-approximation algorithm within  $O(n)$  queries. Although its factor approximation is quite large, it is the *first deterministic algorithm* that gives a constant approximation factor within only a linear number of queries for the general SMK problem. LA is a key building block for our DLA and its randomized version, RLA.

### 4.1 LA Algorithm

The LA algorithm (Algorithm 1) splits the ground set into two subsets  $V_1$  and  $V_2$ . The first contains any element whose cost is at most  $B/2$ ; the second includes the rest. The key strategy for LA is dividing the ground set into subsets to quickly find out the bound of the optimal solution in linear queries, then

---

#### Algorithm 1: LA Algorithm

---

**Input:** An instance  $(f, V, B)$ .  
1:  $V_1 \leftarrow \{e \in V : c(e) \leq B/2\}$ ,  $X \leftarrow \emptyset$ ,  $Y \leftarrow \emptyset$   
 $e_{max} \leftarrow \arg \max_{e \in V} f(e)$   
2: **foreach**  $e \in V_1$  **do**  
3: Find  $Z \in \{X, Y\}$  such that:  
 $Z = \arg \max_{Z \in \{X, Y\}: \frac{f(e|Z)}{c(e)} \geq \frac{f(Z)}{B} \frac{f(e|Z)}{c(e)}}$   
4: **If** exist such set  $Z$  **then**  $Z \leftarrow Z \cup \{e\}$   
5: **end**  
6:  $X' \leftarrow \arg \max_{X(j): 0 \leq j \leq |X|, c(X(j)) \leq B} c(X(j))$   
7:  $Y' \leftarrow \arg \max_{Y(j): 0 \leq j \leq |Y|, c(Y(j)) \leq B} c(Y(j))$ , where  
 $T(j)$  is a set of last  $j$  elements added in  $T \in \{X, Y\}$ .  
8:  $S \leftarrow \arg \max_{Z \in \{X', Y', \{e_{max}\}\}} f(Z)$   
9: **return**  $S$ .

---

selecting potential elements into two sets to get a constant approximation factor for SMK.

Since the feasible solution for over  $V_2$  contains at most one element, we can bound it by the maximal singleton  $e_{max} = \arg \max_{e \in V} f(e)$ . For the subset  $V_1$ , the algorithm initiates two empty disjoint sets  $X, Y$ ; each has a threshold (ratio of  $f$  value over  $B$ ) to consider the admission of a new element. A considered element is added to a set  $Z \in \{X, Y\}$  to which it has the higher ratio between marginal gain and its cost with respect to  $Z$  (i.e. “density gain”) as long as the density gain is at least  $f(Z)/B$ . Note that the cost of disjoint sets may be higher than  $B$ , so we obtain feasible solutions from them by only selecting the last elements added with the cost nearest to  $B$  (lines 6-7). Finally, the algorithm returns a feasible solution with the maximum  $f$  value.

Note that the approach of [Li *et al.*, 2022] gave a range bound of an optimal solution for the **monotone** SMK problem in linear time, but it does not work for the **non-monotone** objective function and does not provide any feasible solution. To deal with the non-monotone function, our algorithm maintains  $X$  and  $Y$  to be always disjoint and exploit (2) to get:

$$f(O_1) \leq f(X \cup O_1) + f(Y \cup O_1).$$

and bound the optimal value by  $f(O) \leq f(O_1) + f(O_2)$  where  $O_1$  and  $O_2$  are optimal solutions of the problem over  $V_1$  and  $V_2$ , respectively.

On the other hand, an advantage of our algorithm is that we can use the  $f$  value of the maximal singleton to design and analyze theoretical bounds for our later algorithms.

Lemma 2 provides a bound of optimal solution  $V_1$  by two disjoint sets  $X, Y$ , which is critical to analyze the theoretical bound of Algorithm 1.

**Lemma 2.** At the end of the main loop of Algorithm 1, we have:  $f(O_1) \leq 3(f(X) + f(Y))$ .

**Theorem 1.** Algorithm 1 is deterministic, returns an approximation factor of 19 and takes  $O(n)$  queries.

We further introduce the LAR (Algorithm 2) algorithm, a randomized version of Algorithm 1. LAR selects  $V_p$  from  $V_1$  by selecting  $e \in V_1$  with probability  $p > 0$ , then it builds the candidate set  $S$  from  $V_p$  instead of maintaining two disjoint

---

**Algorithm 2: LAR Algorithm**

---

**Input:** An instance  $(f, V, B)$ , parameters  $p, \alpha$

- 1:  $e_{max} \leftarrow \max_{e \in V} f(e)$ ,  $V_1 \leftarrow \{e \in V | c(e) \leq B/2\}$
- 2:  $V_p \leftarrow \{e \in V_1 : \text{Select } e \text{ with probability } p\}$ ,  $S \leftarrow \emptyset$
- 3: **foreach**  $e \in V_p$  **do**
- 4:   **If**  $f(e|S)/c(e) \geq \alpha f(S)/B$  **then**  $S \leftarrow S \cup \{e\}$
- 5: **end**
- 6:  $S' \leftarrow \arg \max_{S(j): 0 \leq j \leq |X|, c(X(j)) \leq B} c(S(j))$ , where  $S(j)$  is a set of last  $j$  elements added into  $S$ .
- 7:  $S \leftarrow \arg \max_{T \in \{S', \{e_{max}\}\}} f(T)$
- 8: **return**  $S$ .

---

sets. Although LAR is a randomized algorithm, it provides a better approximation factor of LA and be used for designing a later randomized algorithm RLA.

**Theorem 2.** *Algorithm 2 takes  $O(n)$  queries and returns an approximation factor of 16.034 with  $p = \sqrt{2} - 1$  and  $\alpha = \sqrt{2} + 2\sqrt{2}$ .*

Due to space limit, proofs of Lemmas, Theorems 1 and 2 are provided in the Appendix.

## 4.2 DLA Algorithm

We now introduce our DLA (Algorithm 3), a **D**eterministic and **L**inear query complexity **A**pproximation algorithm that has an approximation factor of  $6 + \epsilon$ . The key strategy is combining the properties of two disjoint sets with a greedy threshold to construct several candidate solutions to analyze the theory of the non-monotone objective function.

DLA takes an instance  $(f, V, B)$  and a parameter  $\epsilon$  as inputs. DLA consists of two phases. At the first one (lines 1-9), the algorithm calls LA as a subroutine to obtain a candidate solution  $S'$  and get an approximate range of optimal value  $[\Gamma, 19\Gamma]$  where  $\Gamma = f(S')$  (line 1). It then adapts the greedy threshold to add elements with high-density gain into two disjoint sets  $X$  and  $Y$ . Specifically, this phase consists of multiple iterations; each scans one time over the ground set (lines 3-9). An element added to the set  $T \in \{X, Y\}$  to which has the higher density gain without violating the budget constraint, as long as the density gain is at least  $\theta$ , which initiates to  $19\Gamma/(6\epsilon')$  and decreases by a factor of  $(1 - \epsilon')$  after each iteration until less than to  $\Gamma(1 - \epsilon')/(6B)$ , where  $\epsilon' = \epsilon/14$ .

The second phase (lines 10-16) is to improve the quality of candidate solution  $T \in \{X, Y\}$  which was obtained at the end of phase 1. Denote  $T^i$  as a set of the first  $i^{th}$  elements added in  $T$  in phase 1. Our main observation is that the performance of DLA depends on the cost of  $T' = \arg \max_{T^i: c(T^i) \leq B - c(r)} c(T^i)$ . Recall that  $r$  is  $\arg \max_{o \in O} c(o)$  and  $c(r) \leq B$ . We scan an upper bound of  $c(T')$  from  $\epsilon'B$  to  $B$  and improve the quality of  $T'$  by adding into it an element  $e = \arg \max_{e \in V: c(T' \cup \{e\}) \leq B} f(T' \cup \{e\})$  (lines 13-15).

The following Lemmas give the bounds of the final solution when  $c(r) < (1 - \epsilon')B$  and  $c(r) \geq (1 - \epsilon')B$ , respectively.

**Lemma 3.** *If  $c(r) < (1 - \epsilon')B$ , one of two things happens: a)  $f(S) \geq \frac{1}{6(1+\epsilon')} \text{opt}$ ; b) There exists a subset  $X' \subseteq X$  so*

---

**Algorithm 3: DLA Algorithm**

---

**Input:** An instance  $(f, V, B)$ ,  $\epsilon > 0$

- 1:  $S' \leftarrow \text{LA}(f, V, B)$ ,  $\Gamma \leftarrow f(S')$ ,  $\epsilon' \leftarrow \frac{\epsilon}{14}$
- 2:  $\Delta \leftarrow \lceil \frac{\log(1/\epsilon')}{\epsilon'} \rceil$ ,  $\theta \leftarrow 19\Gamma/(6\epsilon'B)$ ,  $X \leftarrow \emptyset$ ,  $Y \leftarrow \emptyset$
- 3: **while**  $\theta \geq \Gamma(1 - \epsilon')/(6B)$  **do**
- 4:   **foreach**  $e \in V \setminus (X \cup Y)$  **do**
- 5:     Find  $T \in \{X, Y\}$  such that:  $c(T \cup \{e\}) \leq B$   
and  $T = \arg \max_{T \in \{X, Y\}, \frac{f(e|T)}{c(e)} \geq \theta} \frac{f(e|T)}{c(e)}$
- 6:     **If** exist such set  $T$  **then**  $T \leftarrow T \cup \{e\}$
- 7:   **end**
- 8:    $\theta \leftarrow (1 - \epsilon')\theta$
- 9: **end**
- 10: **for**  $l = 0$  **to**  $\Delta$  **do**
- 11:    $X'_{(l)} \leftarrow \arg \max_{X^i: c(X^i) \leq \epsilon'B(1+\epsilon')^l, i \leq |X|} i$
- 12:    $Y'_{(l)} \leftarrow \arg \max_{Y^i: c(Y^i) \leq \epsilon'B(1+\epsilon')^l, i \leq |Y|} i$
- 13:    $e_X \leftarrow \arg \max_{e \in V: c(X'_{(l)} \cup \{e\}) \leq B} f(X'_{(l)} \cup \{e\})$
- 14:    $e_Y \leftarrow \arg \max_{e \in V: c(Y'_{(l)} \cup \{e\}) \leq B} f(Y'_{(l)} \cup \{e\})$
- 15:    $X_{(l)} \leftarrow X'_{(l)} \cup \{e_X\}$ ,  $Y_{(l)} \leftarrow Y'_{(l)} \cup \{e_Y\}$
- 16: **end**
- 17:  $S \leftarrow \arg \max_{T \in \{S', X, Y, X_{(0)}, \dots, X_{(\Delta)}, Y_{(0)}, \dots, Y_{(\Delta)}\}} f(T)$
- 18: **return**  $S$ .

---

that  $f(O \cup X') \leq 2f(S) + \max\{\frac{1+\epsilon'}{1-\epsilon'} f(S), \frac{(1-\epsilon')}{6} \text{opt}\}$ . Similarly, one of two conditions happens: **c)**  $f(S) \geq \frac{1}{6(1+\epsilon')} \text{opt}$ ; **d)** There exists a subset  $Y' \subseteq Y$  so that  $f(O \cup Y') \leq 2f(S) + \max\{\frac{1+\epsilon'}{1-\epsilon'} f(S), \frac{(1-\epsilon')}{6} \text{opt}\}$ .

**Lemma 4.** *If  $c(r) \geq (1 - \epsilon')B$ , one of two things happens: **e)**  $f(S) \geq \frac{(1-\epsilon')^2}{6} \text{opt}$ ; **f)** There exists a subset  $X' \subseteq X$  so that  $f(O \cup X') \leq 2f(S) + \max\{\frac{(1-\epsilon') \text{opt}}{6}, f(S) + \frac{\epsilon' \text{opt}}{6}\}$ . Similarly, one of two things happens: **g)**  $f(S) \geq \frac{(1-\epsilon')^2}{6} \text{opt}$ ; **h)** There exists a subset  $Y' \subseteq Y$  so that  $f(O \cup Y') \leq 2f(S) + \max\{\frac{(1-\epsilon') \text{opt}}{6}, f(S) + \frac{\epsilon' \text{opt}}{6}\}$ .*

**Theorem 3.** *For any  $\epsilon \in (0, 1)$ , DLA is a deterministic algorithm that has a query complexity  $O(n \log(1/\epsilon)/\epsilon)$  and returns an approximation factor of  $6 + \epsilon$ .*

*Proof.* The query complexity of Algorithm 3 is obtained by combining the operation of Algorithm 1 and two main loops of Algorithm 3. The first and the second loops contain at most  $\lceil \log(19/\epsilon')/\epsilon' \rceil + 1$  and  $\lceil \log(1/\epsilon')/\epsilon' \rceil$  iterations, respectively. Each iteration of these loops takes  $O(n)$  queries; thus we get the total number of queries at most:

$$3n + n(\lceil \frac{1}{\epsilon'} \log(\frac{19}{\epsilon'}) \rceil + 1) + n\lceil \frac{1}{\epsilon'} \log(\frac{1}{\epsilon'}) \rceil = O(\frac{n}{\epsilon} \log(\frac{1}{\epsilon})).$$

To prove the factor, we consider two following cases:

**Case 1.** If  $c(r) \geq (1 - \epsilon')B$ . By using Lemma 4, we consider two cases: If **e)** or **g)** happens. Since  $\epsilon' = \frac{\epsilon}{14} < \frac{1}{14}$  we get:  $\text{opt} \leq \frac{6f(S)}{(1-\epsilon')^2} \leq 6(1 + \frac{14}{13}\epsilon')^2 f(S) < (6 + \epsilon)f(S)$ , the Theorem holds. We consider the otherwise case: both **e)** and **h)** happen. There exist  $X' \subseteq X$ ,  $Y' \subseteq Y$  and  $X' \cap Y' = \emptyset$

satisfying:  $\text{opt} = f(O) \leq f(O \cup X') + f(O \cup Y')$

$$\leq 4f(S) + 2 \max\{(1 - \epsilon')\text{opt}/6, f(S) + \epsilon'\text{opt}/6\}. \quad (3)$$

We consider two sub-cases: If  $f(S) \geq \frac{\text{opt}}{6}$ , the Theorem holds. If  $f(S) < \frac{\text{opt}}{6}$ , put it back into (3) we get:

$$\text{opt} < 4f(S) + \frac{1+\epsilon'}{3}\text{opt} \Rightarrow \text{opt} \leq \frac{12f(S)}{2-\epsilon'} < (6 + \epsilon)f(S).$$

**Case 2.** If  $c(r) < (1 - \epsilon')B$ . By applying the Lemma 3, we consider two cases: If **a)** or **c)** happens, we get  $f(S) \geq \frac{\text{opt}}{6(1+\epsilon')} \Rightarrow \text{opt} \leq (6 + 6\epsilon')f(S)$  and the Theorem holds. If both **b)** and **d)** happen. There exist  $X' \subseteq X, Y' \subseteq Y$  and  $X' \cap Y' = \emptyset$  satisfying:  $\text{opt} = f(O) \leq f(O \cup X') + f(O \cup Y')$

$$\leq 4f(S) + 2 \max\left\{\frac{1+\epsilon'}{1-\epsilon'}f(S), \frac{(1-\epsilon')\text{opt}}{6}\right\}. \quad (4)$$

If  $f(S) \geq \frac{\text{opt}}{6}$ , the Theorem is true. We consider the case  $f(S) < \frac{\text{opt}}{6}$ , put it into (4) we get  $\text{opt} < 4f(S) + \frac{1+\epsilon'}{1-\epsilon'}\frac{\text{opt}}{3}$ .

$$\Rightarrow \text{opt} < \frac{6(1-\epsilon')}{1-2\epsilon'}f(S) = (6 + \frac{6\epsilon'}{1-2\epsilon'})f(S) < (6 + \epsilon)f(S).$$

Combining two cases, we obtain the proof.  $\square$

### 4.3 RLA Algorithm

We further introduce the RLA (Algorithm 4), a **R**andomized and **L**inear query complexity **A**pproximation algorithm with the factor of  $4 + \epsilon$ . RLA re-uses the algorithmic framework of DLA algorithm with some modifications. In particular, we combine the threshold greedy method with a random process to construct a series of candidate solutions  $S_j$ .

Specifically, the first phase of the algorithm consists of a loop (lines 2-11) with at most  $\lceil \log(4/\epsilon')/\epsilon' \rceil$  iterations, and each takes one pass over the ground set, where  $\epsilon' = \epsilon/10$ . This loop simultaneously constructs a *candidate set*  $U = \{u_1, \dots, u_j\}$  and a solution  $S_j$  as follows: Each element  $e$ , not in the current candidate set, having the density gain at least  $\theta$ , is added into the candidate set and then added into  $S_{j+1}$  with probability  $1/2$ . The set  $U$  plays an important role to the RLA's performance. In the second phase of this algorithm, we boost the quality of candidate solution  $S_j$  by using the same strategy with the DLA (lines 12-16).

We now analyze the performance of RLA. Considering the end of the algorithm, we first define the following notations: For any  $u_i \in U = \{u_1, u_2, \dots, u_j\}$ , define  $\tau(u_i) = i$ ,  $S^{<u_i} = S_{i-1}$ ; for any  $e \in V \setminus U$ ,  $\tau(e) = +\infty$ . Denote  $T = j$ , if  $c(S_{j-1} \cup \{u_j\}) \leq B - c(r)$ . Otherwise,  $T = \min\{i : 0 \leq i \leq j-1, c(S_i \cup \{u_{i+1}\}) > B - c(r)\}$ . Lemma 5 provides an efficient tool to estimate  $f(S_i)$  for all  $i \leq j$  that is helpful to obtain RLA's performance guarantee.

**Lemma 5.** For each  $u_i \in \{u_1, \dots, u_j\}$ , we define:  $O_{\leq i} = \{e : e \in O, \tau(e) \leq i\}$ ,  $O_{> i} = \{e : e \in O, \tau(e) > i\}$  and

$$X_e = \begin{cases} 1, e \in O_{\leq i} \setminus S_i \text{ or } e \in S_i \setminus O \\ 0, \text{otherwise.} \end{cases}$$

$$Y_e = \begin{cases} 1, e \in O_{\leq i} \setminus (S_i \cup \{r\}) \text{ or } u \in S_i \setminus (O \setminus \{r\}) \\ 0, \text{otherwise.} \end{cases}$$

a) For any  $S_i$  we have  $\mathbb{E}[f(S_i)] = \mathbb{E}[\sum_{e \in V} X_e \cdot f(e|S^{<e})]$ .

b) For any  $S_i$  satisfying  $c(S_i) \leq B - c(r)$  we have  $\mathbb{E}[f(S_i)] = \mathbb{E}[\sum_{e \in V} Y_e \cdot f(e|S^{<e})]$ .

---

#### Algorithm 4: RLA Algorithm

---

**Input:** An instance  $(f, V, B), \epsilon > 0$

```

1:  $S' \leftarrow \text{LAR}(f, V, B, p = \sqrt{2} - 1, \alpha = \sqrt{2 + 2\sqrt{2}})$ ,
    $S_j \leftarrow \emptyset, j \leftarrow 0, \Gamma \leftarrow f(S'), \theta \leftarrow \frac{16.034\Gamma}{4\epsilon'B}, \epsilon' \leftarrow \frac{\epsilon}{10}$ 
2: while  $\theta \geq \Gamma(1 - \epsilon')/(4B)$  do
3:   foreach  $e \in V \setminus \{u_1, u_2, \dots, u_j\}$  do
4:     if  $\frac{f(e|S_j)}{c(e)} \geq \theta$  and  $c(S_j) + c(e) \leq B$  then
5:        $u_j \leftarrow e$ ;
6:       With probability  $1/2$  do:
7:          $S_{j+1} \leftarrow S_j \cup \{e\}$  otherwise  $S_{j+1} \leftarrow S_j$ 
8:        $j \leftarrow j + 1$ 
9:   end
10:   $\theta \leftarrow (1 - \epsilon')\theta$ 
11: end
12: for  $l = 0$  to  $\lceil \log(1/\epsilon')/\epsilon' \rceil$  do
13:    $S'_{(l)} \leftarrow \arg \max_{S_i: c(S_i) \leq \epsilon'B(1+\epsilon')^l, i \leq |S|} f(S_i)$ 
14:    $e_{max}^l \leftarrow \arg \max_{e \in V: c(S'_{(l)} \cup \{e\}) \leq B} f(S'_{(l)} \cup \{e\})$ 
15:    $S_{(l)} \leftarrow S'_{(l)} \cup \{e_{max}^l\}$ 
16: end
17:  $S \leftarrow \arg \max_{X \in \{S', S_j, S_{(0)}, \dots, S_{(\lceil \log(1/\epsilon')/\epsilon' \rceil)}\}} f(X)$ 
18: return  $S$ .
```

---

**Theorem 4.** For any  $\epsilon \in (0, 1)$ , RLA is a randomized algorithm with query complexity of  $O(n \log(1/\epsilon)/\epsilon)$  and returns an approximation ratio of  $4 + \epsilon$  in expectation.

*Proof.* The query complexity of RLA is obtained by the same argument in the proof of Theorem 3. Denote by  $\theta_i$   $\theta$  at the iteration  $i$ , by  $\theta_{(i)}$   $\theta$  when  $u_i$  is added into  $U$ , and  $\theta_{last}$  is  $\theta$  at the last iteration of the first loop. For the approximation factor, we consider the following cases:

**Case 1.** If  $c(r) > (1 - \epsilon')B$ ,  $c(O \setminus \{r\}) < B - (1 - \epsilon')B = \epsilon'B$ . We consider two following sub-cases: **Case 1.1.** If  $c(S_j) \geq (1 - \epsilon')B$ , then  $f(S) \geq f(S_j) \geq c(S_j)(1 - \epsilon')\frac{\text{opt}}{4} \geq (1 - \epsilon')^2\frac{\text{opt}}{4}$ . Since  $\epsilon' = \frac{\epsilon}{10} < \frac{1}{10}$ , we have:  $\text{opt} \leq \frac{4f(S)}{(1-\epsilon')^2} \leq 4(1 + \frac{10}{9}\epsilon')^2 f(S) \leq (4 + \epsilon)f(S)$ . **Case 1.2.** If  $c(S_j) < (1 - \epsilon')B$ ,  $c(S_j) + c(e) \leq c(S_j) + c(O \setminus \{r\}) < B$  for all  $e \in (O \setminus \{r\}) \setminus S_j$ . Thus  $\frac{f(e|S_j)}{c(e)} < \frac{(1-\epsilon')\Gamma}{4B} \leq \frac{(1-\epsilon')\text{opt}}{4B}$ .

$$\Rightarrow f((O \setminus \{r\}) \cup S_j) - f(S_j) \leq \sum_{e \in (O \setminus \{r\}) \setminus S_j} f(e|S_j) < c(O \setminus \{r\})(1 - \epsilon')\text{opt}/(4B) \leq \epsilon'(1 - \epsilon')\text{opt}/4. \quad (5)$$

Since each element in  $V$  appears in  $S_j$  with probability  $1/2$ , applying Lemma 1 gives  $\mathbb{E}[f(O \setminus \{r\} \cup S_j)] \geq \frac{1}{2}f(O \setminus \{r\})$ . Combine this with (5), we have:  $f(O) \leq f(O \setminus \{r\}) + f(r) \leq 2\mathbb{E}[f(O \setminus \{r\} \cup S_j)] + f(e_{max}) < 3\mathbb{E}[f(S)] + \frac{\epsilon'(1-\epsilon')\text{opt}}{2}$ .

$$\Rightarrow \text{opt} < \frac{6\mathbb{E}[f(S)]}{2 - \epsilon'(1 - \epsilon')} \leq \frac{6\mathbb{E}[f(S)]}{2 - \epsilon'} \leq (4 + \epsilon)\mathbb{E}[f(S)].$$

**Case 2.** If  $c(r) \leq (1 - \epsilon')B$ ,  $c(O \setminus \{r\}) \geq \epsilon'B$ . Considering the following sub-cases: **Case 2.1.** If  $T = j$ , by the definition

of  $T$  we have:  $O_{>T} = \emptyset$ . Therefore

$$\begin{aligned} f(S_T \cup O) - f(S_T) &\leq \sum_{e \in O_{\leq T} \setminus S_T} f(e|S_T) \\ &\leq \sum_{e \in O_{\leq T} \setminus S_T} f(e|S^{<e}) + \sum_{e \in S_T \setminus O} f(e|S^{<e}) \end{aligned} \quad (6)$$

$$= \sum_{e \in V} X_e \cdot f(e|S^{<e}) = \mathbb{E}[f(S_T)]. \quad (7)$$

where (6) due to  $f(e|S^{<e}) > 0, \forall e \in S_j$  and  $X_e$  is defined in Lemma 5. By applying Lemma 1 again, we have  $\mathbb{E}[f(O \cup S_T)] \geq f(O)/2$ . Combine this with (7), we attain

$$\mathbb{E}[f(S)] \geq \mathbb{E}[f(S_T)] \geq \mathbb{E}[f(O \cup S_T)]/2 \geq f(O)/4.$$

**Case 2.2.** If  $T < j$ ,  $U$  contains at least  $T+1$  elements and we have  $c(S_T) + c(u_{T+1}) > B - c(r) > \epsilon' B$ . We now consider the second loop of the Algorithm 3. Since  $\epsilon' B < B - c(r) \leq B$ , there exists an integer number  $l$  that:

$$\epsilon' B \leq (1 + \epsilon')^l \epsilon' B \leq B - c(r) < (1 + \epsilon')^{l+1} \epsilon' B.$$

Assuming that  $S'_{(l)} = S_i$  for some  $i$ . By selection rule of  $S'_{(l)}$  we have  $c(S_i) \leq (1 + \epsilon')^l \epsilon' B < c(S_i \cup \{u_{i+1}\})$  thus  $c(S_i \cup \{u_{i+1}\}) > \frac{\epsilon' B}{1 + \epsilon'}$ . We further consider two sub-cases.

If  $u_{i+1}$  is considered at the first iteration of the first loop, by the selection rule of  $e_{max}^l$  at the second loop, we get:

$$f(S_{(l)}) \geq f(S_i \cup \{u_{i+1}\}) \geq c(S_i \cup \{u_{i+1}\})\theta_1 \geq \frac{\text{opt}}{4(1 + \epsilon')^2}.$$

Hence,  $\text{opt} \leq 4(1 + \epsilon')^2 f(S) < (4 + \epsilon) f(S)$ .

If  $u_{i+1}$  is considered at the  $l^{\text{th}}$  iteration,  $l \geq 2$ . Let  $\hat{S} = S_i \setminus (O \setminus \{r\})$  and  $\hat{O} = O_{\leq i} \setminus (S_i \cup \{r\})$ . We show that

$$c(\hat{S}) + c(u_{i+1}) > c(O_{>i} \setminus \{r\}). \quad (8)$$

$$\begin{aligned} \text{Indeed, } c(S_i \setminus (O \setminus \{r\})) + c(S_i \cap (O \setminus \{r\})) + c(u_{i+1}) \\ = c(S_i) + c(u_{i+1}) > B - c(r) \geq c(O \setminus \{r\}) \\ \geq c(O_{>i} \setminus \{r\}) + c(S_i \cap (O \setminus \{r\})). \end{aligned}$$

thus (8) is true. On the other hand, for any element  $e \in O_{>i} \setminus \{r\}$ , its density gain with respect to  $S_i$  is smaller than the threshold at the previous iteration (in the first loop), i.e.,  $\frac{f(e|S_i)}{c(e)} \leq \frac{\theta_{(i+1)}}{1 - \epsilon'}$ . Combine this with (8), we obtain:

$$\begin{aligned} \sum_{e \in O_{>i} \setminus \{r\}} f(e|S_i) &= \sum_{e \in O_{>i} \setminus \{r\}} \frac{f(e|S_i)}{c(e)} c(e) \\ &\leq \frac{c(O_{>i} \setminus \{r\})\theta_{(i+1)}}{1 - \epsilon'} < \frac{c(\hat{S} \cup \{u_{i+1}\})\theta_{(i+1)}}{1 - \epsilon'} \\ &\leq \frac{\sum_{e \in \hat{S} \cup \{u_{i+1}\}} f(e|S^{<e})}{1 - \epsilon'} \end{aligned} \quad (9)$$

where (9) due to the reason that  $\frac{f(e|S^{<e})}{c(e)} \geq \theta_{(i+1)}, \forall e \in S_i \cup \{u_{i+1}\}$ , thus  $\sum_{e \in \hat{S} \cup \{u_{i+1}\}} f(e|S^{<e}) \geq c(\hat{S} \cup \{u_{i+1}\})\theta_{(i+1)}$ .

$$\begin{aligned} \implies f(S_i \cup O) - f(S_i \cup \{r\}) &\leq \sum_{e \in O \setminus (S_i \cup \{r\})} f(e|S_i) \\ &= \sum_{e \in \hat{O}} f(e|S_i) + \sum_{e \in O_{>i} \setminus \{r\}} f(e|S_i) \\ &< \frac{\sum_{e \in \hat{O}} f(e|S^{<e}) + \sum_{e \in \hat{S}} f(e|S^{<e}) + f(u_{i+1}|S_i)}{1 - \epsilon'} \end{aligned}$$

$$\leq \frac{Y_e \cdot f(e|S^{<e}) + f(e_{max}^l|S_i)}{1 - \epsilon'} \quad (10)$$

where  $Y_e$  is defined in Lemma 5. From (10) and by applying Lemma 5, we have:

$$\begin{aligned} \mathbb{E}[f(S_i \cup O)] &< \frac{\mathbb{E}[f(S_i)] + \mathbb{E}[f(e_{max}^l|S_i)]}{1 - \epsilon'} + \\ \mathbb{E}[f(S_i \cup \{r\})] &\leq \frac{\mathbb{E}[f(S)]}{1 - \epsilon'} + \mathbb{E}[f(S)] = \frac{2 - \epsilon'}{1 - \epsilon'} \mathbb{E}[f(S)]. \end{aligned}$$

By applying Lemma 1, we have  $f(O) \leq 2\mathbb{E}[f(S_i \cup O)]$ . Thus

$$f(O) < \frac{2(2 - \epsilon')}{1 - \epsilon'} \mathbb{E}[f(S)] \leq (4 + \epsilon) \mathbb{E}[f(S)].$$

By combining all cases, we attain the proof.  $\square$

## 5 Experimental Evaluation

In this section, we compare the performance between our algorithms and state-of-the-art algorithms for the SMK problem on three applications: Revenue Maximization, Image Summarization, and Maximum Weighted Cut.

### 5.1 Applications And Datasets

**Revenue Maximization.** Given a social network that represented by a graph  $G = (V, E)$  where  $V$  and represent a set of users a set of user connections, respectively Each edge  $(u, v)$  assigned a weight  $w_{(u,v)}$  that reflects the “closeness” of  $u$  and  $v$ . We follow [Mirzasoleiman *et al.*, 2016] to define the advertising revenue of any node set  $S \subseteq V$  as  $f(S) = \sum_{u \in V \setminus S} \sqrt{\sum_{v \in S: (v,u) \in E} w_{(u,v)}}$ . The weight  $w_{(u,v)}$  is randomly sampled from the continuous uniform distribution  $U(0, 1)$  as in and each node  $u$  has a cost  $c(u) = g(\sqrt{\sum_{(u,v) \in E} w_{(u,v)}})$  where  $g(x) = 1 - e^{-\mu x}$  and  $\mu = 0.2$  [Han *et al.*, 2021]. Given a budget of  $B$ , the goal of the problem is to select a set  $S$  with the cost at most  $B$  to maximize  $f(S)$ . This problem is an instance of non-monotone SMK [Han *et al.*, 2021]. In this application, we utilized the ego-Facebook dataset from [Leskovec *et al.*, 2007] which consists of over 4K nodes and over 88K edges.

**Image Summarization.** Given a graph  $G = (V, E)$  where each node  $u \in V$  represents an image, and each edge  $(u, v) \in E$  is assigned a weight  $w_{u,v}$  representing the similarity between image  $u$  and image  $v$ . Define  $c(u)$  the cost to collect the image  $u$ . The goal is to identify a representative subset  $S \subseteq V$  with a limited budget  $B$  that maximizes the representative value defined as  $f(S) = \sum_{u \in V} \max_{v \in S} w_{u,v} - \frac{1}{|V|} \sum_{u \in V} \sum_{v \in S} w_{u,v}$  [Mirzasoleiman *et al.*, 2016; Han *et al.*, 2021]. The function  $f(\cdot)$  is non-monotone, non-negative, and submodular [Mirzasoleiman *et al.*, 2016]. Following the recent work [Han *et al.*, 2021; Mirzasoleiman *et al.*, 2016], we set this instance as follows: We first randomly selected 500 images from the CIFAR data sets [Krizhevsky, 2019; Mirzasoleiman *et al.*, 2016], which contained 10,000 images. We then measure the similarity between image  $u$  and image  $v$  by using the cosine similarity of their 3.072-dimensional pixel vectors. Finally, we use Root Mean Square (RMS) contrast as a metric to evaluate the quality of the images and assign a cost to each image based on its RMS contrast.

**Maximum Weighted Cut.** Given a graph  $G = (V, E)$ , and a non-negative edge weight  $w_{u,v}$  for each  $(u, v) \in E$ . For a set of nodes  $S \subset V$ , define the weighted cut function  $f(S) = \sum_{u \in V \setminus S} \sum_{v \in S} w_{u,v}$ . The maximum (weighted) cut problem is to find a subset  $S \subseteq V$  such that the  $f(S)$  is maximized. It is indicated in [Kuhnle, 2019; Amanatidis *et al.*, 2020] as  $f(\cdot)$  is non-monotone and submodular. The datasets used in the application included an Erdős-Rényi (ER) random graph with 5000 nodes, and an edge probability of 0.2 and the cost of each node  $c(u)$  was randomly uniformly chosen from the range  $(0, 1)$  as in [Amanatidis *et al.*, 2020].

**Experiment Settings.** We compare our algorithms with the applicable state-of-the-art algorithms listed below:

- **FANTOM:** The randomized algorithm of [Mirzasoileman *et al.*, 2016] with the expected factor of the  $10 + \epsilon$  in  $O(n^2 \log(n)/\epsilon)$ .
- **SAMPLE GREEDY:** The randomized algorithm of [Amanatidis *et al.*, 2020] with the factor  $5.83 + \epsilon$  in query complexity of  $O(n \log(n/\epsilon)/\epsilon)$  queries. For the easy following, we refer to SAMPLE GREEDY as the **GREEDY**.
- **SMKDETACC:** The deterministic algorithm of [Han *et al.*, 2021] with the factor  $6 + \epsilon$  in  $O(n \log(k/\epsilon)/\epsilon)$  queries. This is the fastest deterministic approximation algorithm for non-monotone SMK.
- **SMKRANACC:** This is the fastest randomized algorithm of [Han *et al.*, 2021] with the expected approximation factor  $4 + \epsilon$  in query complexity of  $O(n \log(k/\epsilon)/\epsilon)$ .
- **SMKSTREAM:** The first streaming algorithm for studied problem that returns the approximation factor of  $6 + \epsilon$  within  $O(n \log(B)/\epsilon)$  queries [Han *et al.*, 2021].

In our experiments, the budget range from 2% to 12% of the total cost of the ground sets as setting of [Amanatidis *et al.*, 2020]. We set  $\epsilon = 0.1$  for all algorithms and  $\alpha = \beta = 1/6, h = 2, r = 2$  for SMKSTREAM [Han *et al.*, 2021].

## 5.2 Experiment Results

The result of the experiment is shown in Figure 1. First, Figures 1(a)(c)(e) represent the quality of algorithms via values of the objective function on 3 instances. As can be seen, DLA always gives the highest values at all  $B$  milestones in all instances. RLA, SMKRANACC, and SMKSTREAM are not much different. FANTOM results lower while GREEDY provides the lowest. Regarding the deterministic algorithm, DLA is several tens to thousands of units better than SMKDETACC on (a) and (e), especially, several times higher on (c). Regarding the randomized algorithm, our RLA gives as well quality as SMKRANACC. This result insists that our algorithm ensures good performance compared to the algorithms of [Han *et al.*, 2021], which are currently the best. In the end, our algorithm tends to be considerably better than the rest when  $B$ 's values increase.

Figures 1(b)(d)(f) illustrate the number of queries of the above algorithms. FANTOM is the highest, SMKSTREAM is the second, and the remaining is much lower. FANTOM and SMKSTREAM require millions of queries, whereas the

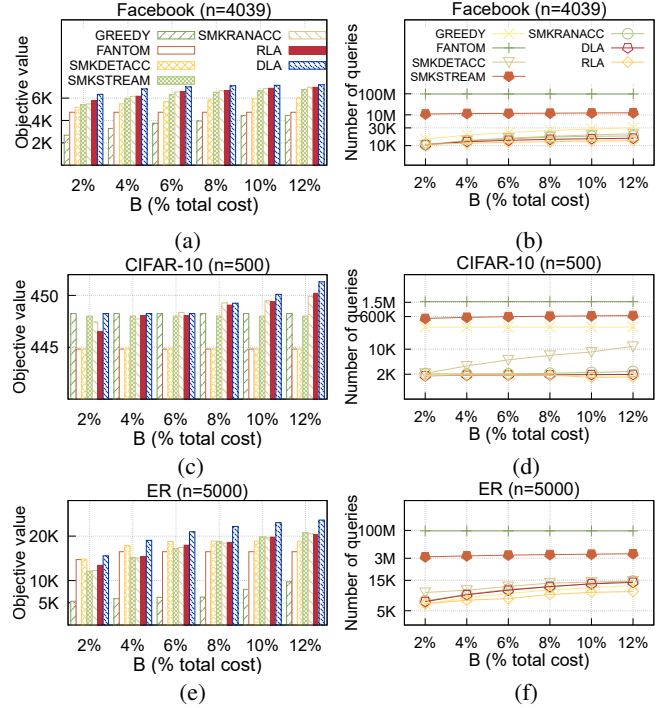

Figure 1: Performance of algorithms for non-monotone SMK on three instances: (a), (b) Revenue Maximization; (c), (d) Image Summarization and (e), (f) Maximum Weighted Cut.

rest is thousands of times lower than them. In the rest, the GREEDY's queries are also usually higher than the others except on (f). Queries of DLA, RLA, and SMKRANACC look similar while queries of SMKDETACC change due to different datasets. RLA spends the fewest queries, and DLA needs fewer queries than that of SMKDETACC. When  $B$  grows, the number of queries of RLA increases slowest, whereas the queries of SMKDETACC increase fastest. Especially, in Image Summarization, DLA, RLA, SMKDETACC, and SMKRANACC are all approximately 2K at  $B = 2\%$  the total cost; however, SMKDETACC is 5 times higher than the rest when  $B = 12\%$ .

On the whole, our algorithms, DLA, and RLA keep the balance between performance guarantee and query complexity. It's extremely important to save running time with big data. Moreover, experimental results show that our algorithms are efficient ones comparable to state-of-the-art algorithms.

## 6 Conclusions

Motivated by the challenge of solving the non-monotone SMK on the massive data, in this work, we proposed two approximation algorithms DLA, RLA. To the best of our knowledge, our algorithms are the first to achieve a constant factor approximation for the considered problem in linear query complexity. Our algorithms' superiority in solution quality and computation complexity compared to state-of-the-art algorithms was supported by the experiment results in three real-world applications.



## Acknowledgements

This work was supported in part by the National Science Foundation (NSF) grants IIS-1908594.

## References

- [Amanatidis *et al.*, 2020] Georgios Amanatidis, Federico Fusco, Philip Lazos, Stefano Leonardi, and Rebecca Reiffenhäuser. Fast adaptive non-monotone submodular maximization subject to a knapsack constraint. In *Annual Conference on Neural Information Processing Systems*, 2020.
- [Amanatidis *et al.*, 2021] Georgios Amanatidis, Federico Fusco, Philip Lazos, Stefano Leonardi, Alberto Marchetti-Spaccamela, and Rebecca Reiffenhäuser. Submodular maximization subject to a knapsack constraint: Combinatorial algorithms with near-optimal adaptive complexity. In *International Conference on Machine Learning*, volume 139 of *Proceedings of Machine Learning Research*, pages 231–242, 2021.
- [Amanatidis *et al.*, 2022] Georgios Amanatidis, Pieter Kleer, and Guido Schäfer. Budget-feasible mechanism design for non-monotone submodular objectives: Offline and online. *Math. Oper. Res.*, 47(3):2286–2309, 2022.
- [Badanidiyuru and Vondrák, 2014] Ashwinkumar Badanidiyuru and Jan Vondrák. Fast algorithms for maximizing submodular functions. In *Annual ACM-SIAM Symposium on Discrete Algorithms*, pages 1497–1514, 2014.
- [Buchbinder and Feldman, 2019] Niv Buchbinder and Moran Feldman. Constrained submodular maximization via a nonsymmetric technique. *Math. Oper. Res.*, 44(3):988–1005, 2019.
- [Buchbinder *et al.*, 2014] Niv Buchbinder, Moran Feldman, Joseph Naor, and Roy Schwartz. Submodular maximization with cardinality constraints. In *Annual ACM-SIAM Symposium on Discrete Algorithms*, pages 1433–1452. SIAM, 2014.
- [Buchbinder *et al.*, 2015] Niv Buchbinder, Moran Feldman, Joseph Naor, and Roy Schwartz. A tight linear time  $(1/2)$ -approximation for unconstrained submodular maximization. In *IEEE Symposium on Foundations of Computer Science*, pages 649–658, 2015.
- [Chekuri *et al.*, 2014] Chandra Chekuri, Jan Vondrák, and Rico Zenklusen. Submodular function maximization via the multilinear relaxation and contention resolution schemes. *SIAM J. Comput.*, 43(6):1831–1879, 2014.
- [Cui *et al.*, 2021] Shuang Cui, Kai Han, Jing Tang, He Huang, Xueying Li, and Zhiyu Li. Streaming algorithms for constrained submodular maximization. *Proc. ACM Meas. Anal. Comput. Syst.*, 6(3):54:1–54:32, 2021.
- [Ene and Nguyen, 2019] Alina Ene and Huy L. Nguyen. A nearly-linear time algorithm for submodular maximization with a knapsack constraint. In *International Colloquium on Automata, Languages, and Programming*, volume 132 of *LIPIcs*, pages 53:1–53:12, 2019.
- [Feldman *et al.*, 2011] Moran Feldman, Joseph Naor, and Roy Schwartz. A unified continuous greedy algorithm for submodular maximization. In *Annual Symposium on Foundations of Computer Science*, pages 570–579, 2011.
- [Gupta *et al.*, 2010] Anupam Gupta, Aaron Roth, Grant Schoenebeck, and Kunal Talwar. Constrained non-monotone submodular maximization: Offline and secretary algorithms. In *International Workshop on Internet and Network Economics*, 2010.
- [Han *et al.*, 2020] Kai Han, Zongmai Cao, Shuang Cui, and Benwei Wu. Deterministic approximation for submodular maximization over a matroid in nearly linear time. In *Advances in Neural Information Processing Systems 33: Annual Conference on Neural Information Processing Systems 2020, NeurIPS 2020*, 2020.
- [Han *et al.*, 2021] Kai Han, Shuang Cui, Tianshuai Zhu, Enpei Zhang, Benwei Wu, Zhizhuo Yin, Tong Xu, Shaojie Tang, and He Huang. Approximation algorithms for submodular data summarization with a knapsack constraint. *Proc. ACM Meas. Anal. Comput. Syst.*, 5(1):05:1–05:31, 2021.
- [Krizhevsky, 2019] Alex Krizhevsky. Learning multiple layers of features from tiny images. *Technical Reports, University of Toronto*, 2019.
- [Kuhnle, 2019] Alan Kuhnle. Interlaced greedy algorithm for maximization of submodular functions in nearly linear time. In *Neural Information Processing Systems*, pages 2371–2381, 2019.
- [Kulik *et al.*, 2013] Ariel Kulik, Hadas Shachnai, and Tami Tamir. Approximations for monotone and nonmonotone submodular maximization with knapsack constraints. *Math. Oper. Res.*, 38(4):729–739, 2013.
- [Lee *et al.*, 2010a] Jon Lee, Vahab S. Mirrokni, Viswanath Nagarajan, and Maxim Sviridenko. Maximizing non-monotone submodular functions under matroid or knapsack constraints. *SIAM J. Discret. Math.*, 23(4):2053–2078, 2010.
- [Lee *et al.*, 2010b] Jon Lee, Vahab S. Mirrokni, Viswanath Nagarajan, and Maxim Sviridenko. Maximizing non-monotone submodular functions under matroid or knapsack constraints. *SIAM J. Discret. Math.*, 23(4):2053–2078, 2010.
- [Leskovec *et al.*, 2007] Jure Leskovec, Andreas Krause, Carlos Guestrin, Christos Faloutsos, Jeanne M. VanBriesen, and Natalie S. Glance. Cost-effective outbreak detection in networks. In *Proc. of the 13th ACM SIGKDD Conf.*, 2007, pages 420–429, 2007.
- [Li *et al.*, 2022] Wenxin Li, Moran Feldman, Ehsan Kazemi, and Amin Karbasi. Submodular maximization in clean linear time. In *Advances in Neural Information Processing Systems*, pages 7887–7897, 2022.
- [Li, 2018] Wenxin Li. Nearly linear time algorithms and lower bound for submodular maximization. *preprint, arXiv:1804.08178*, 2018.



- [Mirzasoleiman *et al.*, 2016] Baharan Mirzasoleiman, Ashwinkumar Badanidiyuru, and Amin Karbasi. Fast constrained submodular maximization: Personalized data summarization. In *International Conference on Machine Learning*, volume 48 of *JMLR Workshop and Conf. Proc.*, pages 1358–1367, 2016.
- [Sun *et al.*, 2022] Xiaoming Sun, Jialin Zhang, Shuo Zhang, and Zhijie Zhang. Improved deterministic algorithms for non-monotone submodular maximization. In Yong Zhang, Dongjing Miao, and Rolf H. Möhring, editors, *Computing and Combinatorics - 28th International Conference, COCOON 2022, Shenzhen, China, October 22-24, 2022, Proceedings*, volume 13595 of *Lecture Notes in Computer Science*, pages 496–507. Springer, 2022.
- [Sviridenko, 2004] Maxim Sviridenko. A note on maximizing a submodular set function subject to a knapsack constraint. *Oper. Res. Lett.*, 32(1):41–43, 2004.
